# Supplementary material for: Benchmark of $\boldsymbol{GW}$ Methods for Core-Level Binding Energies
Source: arXiv:2206.05627 ancillary file (2022-06-11)
Supplement: Supplementary file 1 [file supporting_information.pdf]

# Supporting Information: Benchmark of *GW* Methods for Core-Level Binding Energies

Jiachen Li,[†] Ye Jin,[†] Patrick Rinke,[‡] Weitao Yang,[†] and Dorothea Golze[*,¶,‡]

†*Department of Chemistry, Duke University, Durham, NC 27708, USA*

‡*Department of Applied Physics, Aalto University, Otakaari 1, FI-02150 Espoo, Finland*

¶*Faculty of Chemistry and Food Chemistry, Technische Universität Dresden, 01062 Dresden, Germany*

E-mail: dorothea.golze@tu-dresden.de

## 1 CORE65 results with ev$GW$, $G_{\Delta\mathrm{H}}W_0$ and $G_{RS}W_{RS}$

The labels for the carbon atoms of nitrobenzene and phenylacetylene are used as defined in the SI of Ref. 1. The experimental values are taken from the SI of Ref. 1, where also the citation for each experimental value is listed. The core-level BEs in Table S1 and S2 include the relativistic corrections used in Refs. 1,2.

**Table S1:** Core-level binding energies (BEs) as obtained from ev$GW$@PBE and $G_{\Delta\mathrm{H}}W_0$@PBE. All values in eV. The BEs have been extrapolated to the complete basis set limit by performing a linear regression with respect to the inverse of the total number of basis functions using the cc-pV$n$Z basis set series ($n = 3 - 6$). Relativistic effects are taken into account for both methods.

| CAS | name | formula | core level | ev$GW$@PBE | $G_{\Delta\mathrm{H}}W_0$@PBE | Exp. |
|---|---|---|---|---|---|---|
| 74-82-8 | methane | $CH_4$ | C1s | 292.22 | 290.65 | 290.84 |
| 74-84-0 | ethane | $C_2H_6$ | C1s | 292.09 | 290.75 | 290.71 |
| 74-85-1 | ethene | $C_2H_4$ | C1s | 292.44 | 290.85 | 290.82 |
| 74-86-2 | ethyne | $C_2H_2$ | C1s | 292.89 | 291.22 | 291.25 |
| 630-08-0 | carbon monoxide | CO | O1s | 544.19 | 542.14 | 542.1 |
| 630-08-0 | carbon monoxide | CO | C1s | 297.38 | 295.84 | 296.23 |
| 124-38-9 | carbon dioxide | $CO_2$ | O1s | 543.05 | 540.85 | 541.32 |
| 124-38-9 | carbon dioxide | $CO_2$ | C1s | 298.64 | 297.26 | 297.70 |
| 75-73-0 | tetrafluoromethane | $CF_4$ | F1s | 696.75 | 694.52 | 695.2 |
| 75-73-0 | tetrafluoromethane | $CF_4$ | C1s | 302.74 | 301.25 | 301.90 |
| 593-53-3 | fluoromethane | $CH_3F$ | F1s | 694.04 | 691.97 | 692.4 |
| 593-53-3 | fluoromethane | $CH_3F$ | C1s | 295.04 | 293.54 | 293.56 |
| 75-46-7 | trifluoromethane | $CHF_3$ | F1s | 695.87 | 693.59 | 694.1 |

**Table S1:** Continued

| CAS | name | formula | core level | ev$GW$@PBE | $G_{\Delta H}W_0$@PBE | Exp. |
|---|---|---|---|---|---|---|
| 75-46-7 | trifluoromethane | $CHF_3$ | C1s | 300.32 | 298.77 | 299.16 |
| 67-56-1 | methanol | $CH_3OH$ | O1s | 540.59 | 538.65 | 538.88 |
| 67-56-1 | methanol | $CH_3OH$ | C1s | 293.91 | 292.43 | 292.3 |
| 50-00-0 | formaldehyde | $CH_2O$ | O1s | 541.03 | 539.04 | 539.33 |
| 50-00-0 | formaldehyde | $CH_2O$ | C1s | 296.01 | 294.52 | 294.38 |
| 115-10-6 | dimethyl ether | $CH_3OCH_3$ | O1s | 539.99 | 538.27 | 538.36 |
| 115-10-6 | dimethyl ether | $CH_3OCH_3$ | C1s | 293.65 | 292.19 | 292.17 |
| 64-18-6 | formic acid | HCOOH | O1s (OH) | 542.19 | 540.25 | 540.69 |
| 64-18-6 | formic acid | HCOOH | O1s (C=O) | 540.52 | 538.51 | 539.02 |
| 64-18-6 | formic acid | HCOOH | C1s | 296.96 | 295.46 | 295.75 |
| 67-64-1 | acetone | $(CH_3)_2CO$ | O1s | 539.41 | 537.53 | 537.73 |
| 67-64-1 | acetone | $(CH_3)_2CO$ | C1s (C=O) | 295.01 | 293.62 | 293.88 |
| 67-64-1 | acetone | $(CH_3)_2CO$ | C1s ($CH_3$) | 292.58 | 291.09 | 291.23 |
| 107-31-3 | methyl formate | $HCO_2CH_3$ | O1s ($OCH_3$) | 541.48 | 539.58 | 539.64 |
| 107-31-3 | methyl formate | $HCO_2CH_3$ | O1s (C=O) | 540.06 | 538.00 | 538.24 |
| 64-19-7 | acetic acid | $CH_3COOH$ | O1s (OH) | 541.57 | 539.73 | 540.10 |
| 64-19-7 | acetic acid | $CH_3COOH$ | O1s (C=O) | 539.78 | 537.76 | 538.31 |
| 64-19-7 | acetic acid | $CH_3COOH$ | C1s (COOH) | 296.48 | 295.01 | 295.35 |
| 64-19-7 | acetic acid | $CH_3COOH$ | C1s ($CH_3$) | 293.00 | 291.51 | 291.55 |
| 7732-18-5 | water | $H_2O$ | O1s | 541.43 | 539.45 | 539.7 |
| 10028-15- | ozone | $O_3$ | O1s middle | 548.77 | 546.80 | 546.44 |
| 10028-15- | ozone | $O_3$ | O1s terminal | 543.45 | 541.23 | 541.75 |
| 7782-44-7 | oxygen | $O_2$ | O1s weaker | 546.12 | 543.76 | 544.2 |
| 7782-44-7 | oxygen | $O_2$ | O1s stronger | 545.02 | 542.88 | 543.1 |
| 7727-37-9 | nitrogen | $N_2$ | N1s | 411.42 | 409.87 | 409.93 |
| 7664-41-7 | ammonia | $NH_3$ | N1s | 407.21 | 405.53 | 405.52 |
| 74-90-8 | hydrogen cyanide | HCN | N1s | 408.54 | 406.68 | 406.8 |
| 74-90-8 | hydrogen cyanide | HCN | C1s | 294.81 | 293.34 | 293.5 |
| 75-05-8 | acetonitrile | $CH_3CN$ | N1s | 407.25 | 405.38 | 405.58 |
| 75-05-8 | acetonitrile | $CH_3CN$ | C1s ($CH_3$) | 294.12 | 292.56 | 292.88 |
| 75-05-8 | acetonitrile | $CH_3CN$ | C1s (CN) | 294.03 | 292.36 | 292.60 |
| 56-40-6 | glycine | $C_2H_5NO_2$ | O1s (OH) | 541.68 | 539.71 | 540.2 |
| 56-40-6 | glycine | $C_2H_5NO_2$ | O1s (C=O) | 539.92 | 537.89 | 538.4 |
| 56-40-6 | glycine | $C_2H_5NO_2$ | N1s | 407.06 | 405.20 | 405.4 |
| 56-40-6 | glycine | $C_2H_5NO_2$ | C1s (COOH) | 296.30 | 294.83 | 295.2 |
| 56-40-6 | glycine | $C_2H_5NO_2$ | C1s ($CH_2$) | 293.70 | 292.21 | 292.3 |
| 110-86-1 | pyridine | $C_5H_5N$ | N1s | 406.31 | 404.66 | 404.82 |
| 109-97-7 | pyrrole | $C_4H_4NH$ | N1s | 407.83 | 406.25 | 406.18 |
| 62-53-3 | aniline | $C_6H_5NH_2$ | N1s | 406.85 | 405.09 | 405.31 |
| 57-13-6 | urea | $CO(NH_2)_2$ | O1s | 538.67 | 536.67 | 537.19 |
| 57-13-6 | urea | $CO(NH_2)_2$ | N1s | 407.69 | 405.94 | 406.09 |
| 57-13-6 | urea | $CO(NH_2)_2$ | C1s | 295.98 | 294.49 | 294.84 |
| 74-89-5 | methylamine | $CH_3NH_2$ | N1s | 406.59 | 404.94 | 405.17 |
| 98-95-3 | nitrobenzene | $C_6H_5NO_2$ | O1s | 540.17 | 538.18 | 538.63 |
| 98-95-3 | nitrobenzene | $C_6H_5NO_2$ | N1s | 413.01 | 411.48 | 411.6 |
| 98-95-3 | nitrobenzene | $C_6H_5NO_2$ | C1s (C1) | 293.39 | 291.98 | 292.08 |
| 98-95-3 | nitrobenzene | $C_6H_5NO_2$ | C1s (C2-4) | 292.54 | 291.08 | 291.13 |
| 71-43-2 | benzene | $C_6H_6$ | C1s | 291.85 | 290.38 | 290.38 |
| 536-74-3 | phenylacetylene | $C_8H_6$ | C1s (C3) | 292.49 | 291.05 | 290.88 |
| 536-74-3 | phenylacetylene | $C_8H_6$ | C1s (C2) | 292.05 | 290.57 | 290.55 |
| 536-74-3 | phenylacetylene | $C_8H_6$ | C1s (C4-6) | 291.93 | 290.39 | 290.16 |
| 536-74-3 | phenylacetylene | $C_8H_6$ | C1s (C1) | 291.67 | 290.04 | 289.75 |

**Table S2:** Core-level binding energies as obtained from $G_{\mathrm{RS}}W_{\mathrm{RS}}$@PBE, $G_{\mathrm{RS}}W_{\mathrm{RS}}$@PBE0, $G_{\mathrm{RS}}W_{\mathrm{RS}}$@B3LYP and $G_{\mathrm{RS}}W_{\mathrm{RS}}$@PBEh($\alpha$=0.45). All values in eV. The BEs have been extrapolated to the complete basis set limit by performing a linear regression with respect to the inverse of the total number of basis functions using the cc-pV3Z and cc-pV4Z basis set sets. Relativistic effects are taken into account for all methods.

| name | formula | core level | $G_{\mathrm{RS}}W_{\mathrm{RS}}$@PBE | $G_{\mathrm{RS}}W_{\mathrm{RS}}$@PBE0 | $G_{\mathrm{RS}}W_{\mathrm{RS}}$@B3LYP | $G_{\mathrm{RS}}W_{\mathrm{RS}}$@PBEh($\alpha$=0.45) |
|---|---|---|---|---|---|---|
| methane | $CH_4$ | C1s | 294.73 | 295.11 | 294.85 | 295.50 |
| ethane | $C_2H_6$ | C1s | 294.68 | 295.10 | 294.77 | 295.48 |
| ethene | $C_2H_4$ | C1s | 294.98 | 295.43 | 295.10 | 295.90 |
| ethyne | $C_2H_2$ | C1s | 295.34 | 563.88 | 295.49 | 296.19 |
| carbon monoxide | CO | O1s | 547.78 | 548.01 | 547.53 | 548.26 |
| carbon monoxide | CO | C1s | 299.46 | 300.00 | 299.76 | 300.61 |
| carbon dioxide | $CO_2$ | O1s | 546.78 | 547.17 | 546.65 | 547.59 |
| carbon dioxide | $CO_2$ | C1s | 300.73 | 301.68 | 301.50 | 302.67 |
| tetrafluoromethane | $CF_4$ | F1s | 701.48 | 701.71 | 701.24 | 701.75 |
| tetrafluoromethane | $CF_4$ | C1s | 305.12 | 305.94 | 305.82 | 306.82 |
| fluoromethane | $CH_3F$ | F1s | 699.06 | 699.15 | 698.70 | 699.28 |
| fluoromethane | $CH_3F$ | C1s | 297.53 | 297.94 | 297.74 | 298.44 |
| trifluoromethane | $CHF_3$ | F1s | 700.85 | 701.09 | 700.73 | 701.30 |
| trifluoromethane | $CHF_3$ | C1s | 302.61 | 303.45 | 303.35 | 304.18 |
| methanol | $CH_3OH$ | O1s | 544.63 | 544.85 | 544.34 | 545.12 |
| methanol | $CH_3OH$ | C1s | 296.36 | 296.79 | 296.56 | 297.30 |
| formaldehyde | $CH_2O$ | O1s | 545.13 | 545.36 | 544.87 | 545.59 |
| formaldehyde | $CH_2O$ | C1s | 298.37 | 298.85 | 298.65 | 299.40 |
| dimethyl ether | $CH_3OCH_3$ | O1s | 544.48 | 544.67 | 544.09 | 544.91 |
| dimethyl ether | $CH_3OCH_3$ | C1s | 296.26 | 296.73 | 296.49 | 297.23 |
| formic acid | HCOOH | O1s (OH) | 546.35 | 546.62 | 546.12 | 546.93 |
| formic acid | HCOOH | O1s (C=O) | 544.70 | 544.94 | 544.46 | 545.22 |
| formic acid | HCOOH | C1s | 299.33 | 300.02 | 299.82 | 300.76 |
| acetone | $(CH_3)_2CO$ | O1s | 544.26 | 544.61 | 544.05 | 544.93 |
| acetone | $(CH_3)_2CO$ | C1s (C=O) | 297.62 | 298.19 | 297.93 | 298.80 |
| acetone | $(CH_3)_2CO$ | C1s ($CH_3$) | 295.25 | 295.68 | 295.44 | 296.13 |
| methyl formate | $HCO_2CH_3$ | O1s ($OCH_3$) | 545.81 | 546.10 | 545.52 | 546.38 |
| methyl formate | $HCO_2CH_3$ | O1s (C=O) | 544.29 | 544.62 | 544.11 | 544.92 |
| acetic acid | $CH_3COOH$ | O1s (OH) | 545.84 | 546.17 | 545.66 | 546.50 |
| acetic acid | $CH_3COOH$ | O1s (C=O) | 544.11 | 544.46 | 543.94 | 544.77 |
| acetic acid | $CH_3COOH$ | C1s (COOH) | 298.92 | 299.66 | 299.44 | 300.43 |
| acetic acid | $CH_3COOH$ | C1s ($CH_3$) | 295.65 | 296.09 | 295.83 | 296.55 |
| water | $H_2O$ | O1s | 545.05 | 545.27 | 544.85 | 545.53 |
| ozone | $O_3$ | O1s middle | 552.57 | 553.30 | 552.71 | 554.17 |
| ozone | $O_3$ | O1s terminal | 547.58 | 548.08 | 547.62 | 548.63 |
| oxygen | $O_2$ | O1s weaker | † | † | † | † |
| oxygen | $O_2$ | O1s stronger | † | † | † | † |
| nitrogen | $N_2$ | N1s | 413.99 | 414.20 | 414.07 | 414.88 |
| ammonia | $NH_3$ | N1s | 410.45 | 410.54 | 410.39 | 411.14 |
| hydrogen cyanide | HCN | N1s | 411.68 | 411.88 | 411.68 | 412.58 |
| hydrogen cyanide | HCN | C1s | 297.10 | 297.36 | 297.43 | 297.91 |
| acetonitrile | $CH_3CN$ | N1s | 410.92 | 411.53 | 410.91 | 411.58 |
| acetonitrile | $CH_3CN$ | C1s ($CH_3$) | 296.68 | 297.02 | 296.84 | 297.54 |
| acetonitrile | $CH_3CN$ | C1s (CN) | 296.37 | 296.82 | 296.53 | 297.48 |
| glycine | $C_2H_5NO_2$ | O1s (OH) | 545.97 | 546.20 | 545.70 | 546.55 |
| glycine | $C_2H_5NO_2$ | O1s (C=O) | 545.02 | 545.41 | 544.67 | 543.92 |
| glycine | $C_2H_5NO_2$ | N1s | 410.64 | 410.98 | 410.51 | 411.38 |
| glycine | $C_2H_5NO_2$ | C1s (COOH) | 298.92 | 299.58 | 299.33 | 300.29 |
| glycine | $C_2H_5NO_2$ | C1s ($CH_2$) | 296.49 | 296.77 | 296.67 | 297.37 |

**Table S2:** Continued

| name | formula | core level | $G_{RS}W_{RS}$@PBE | $G_{RS}W_{RS}$@PBE0 | $G_{RS}W_{RS}$@B3LYP | $G_{RS}W_{RS}$@PBEh($\alpha$=0.45) |
|---|---|---|---|---|---|---|
| pyridine | $C_5H_5N$ | N1s | 410.36 | 410.81 | 410.29 | 411.31 |
| pyrrole | $C_4H_4NH$ | N1s | 411.60 | 411.94 | 411.43 | 412.42 |
| aniline | $C_6H_5NH_2$ | N1s | 410.64 | 410.97 | 410.50 | 411.23 |
| urea | $CO(NH_2)_2$ | O1s | 543.03 | 543.32 | 542.80 | 543.60 |
| urea | $CO(NH_2)_2$ | N1s | 411.18 | 411.62 | 411.25 | 412.05 |
| urea | $CO(NH_2)_2$ | C1s | 298.48 | 299.22 | 299.00 | 300.05 |
| methylamine | $CH_3NH_2$ | N1s | 410.25 | 410.55 | 410.10 | 410.93 |
| nitrobenzene | $C_6H_5NO_2$ | O1s | 544.96 | 545.40 | 544.85 | 545.69 |
| nitrobenzene | $C_6H_5NO_2$ | N1s | 416.71 | 417.71 | 417.14 | 418.39 |
| nitrobenzene | $C_6H_5NO_2$ | C1s (C1) | 296.49 | 297.02 | 296.65 | 297.45 |
| nitrobenzene | $C_6H_5NO_2$ | C1s (C2-4) | 295.59 | 296.10 | 295.74 | 296.51 |
| benzene | $C_6H_6$ | C1s | 294.73 | 295.28 | 294.84 | 295.56 |
| phenylacetylene | $C_8H_6$ | C1s (C3) | 295.48 | 295.95 | 295.58 | 296.29 |
| phenylacetylene | $C_8H_6$ | C1s (C2) | 294.94 | 295.42 | 295.06 | 295.74 |
| phenylacetylene | $C_8H_6$ | C1s (C4-6) | 294.93 | 295.41 | 295.04 | 295.78 |
| phenylacetylene | $C_8H_6$ | C1s (C1) | 294.86 | 295.48 | 294.98 | 295.51 |

## 2 ev*GW* results without relativistic correction

**Table S3:** Non-relativistic core-level binding energies from ev*GW*@PBE using the cc-pV*n*Z basis set series with $n = 3-6$. Extrapolated values ($\infty$),standard error (SE) and correlation coefficient $R^2$. The last column indicates the basis sets used for the extrapolation; for most cases all data points ($n = 3-6$) are included; see SI of Ref. 1 for a discussion why $n = 5, 6$ are sometimes excluded. All values in eV.

| | | | | ev*GW*@PBE | | | | | | | |
|---|---|---|---|---|---|---|---|---|---|---|---|
| CAS | name | formula | core level | $n=3$ | $n=4$ | $n=5$ | $n=6$ | $\infty$ | SE | $R^2$ | $n$ used |
| 74-82-8 | methane | $CH_4$ | C1s | 291.59 | 291.83 | 291.90 | 292.08 | 292.11 | 0.94 | 0.05 | 3-6 |
| 74-84-0 | ethane | $C_2H_6$ | C1s | 291.42 | 291.68 | 291.75 | 291.94 | 291.97 | 0.93 | 0.06 | 3-6 |
| 74-85-1 | ethene | $C_2H_4$ | C1s | 291.72 | 291.99 | 292.08 | 292.27 | 292.32 | 0.96 | 0.06 | 3-6 |
| 74-86-2 | ethyne | $C_2H_2$ | C1s | 292.18 | 292.40 | 292.53 | 292.74 | 292.77 | 0.92 | 0.08 | 3-6 |
| 630-08-0 | carbon monoxide | CO | O1s | 543.56 | 543.64 | 543.61 | 543.73 | 543.77 | 0.98 | 0.02 | 3,4,6 |
| 630-08-0 | carbon monoxide | CO | C1s | 296.79 | 297.00 | 297.04 | 297.21 | 297.26 | 0.92 | 0.06 | 3-6 |
| 124-38-9 | carbon dioxide | $CO_2$ | O1s | 542.25 | 542.36 | 542.37 | 542.57 | 542.62 | 0.94 | 0.07 | 3,4,6 |
| 124-38-9 | carbon dioxide | $CO_2$ | C1s | 297.82 | 298.10 | 298.22 | 298.43 | 298.52 | 0.95 | 0.07 | 3-6 |
| 75-73-0 | tetrafluoromethane | $CF_4$ | F1s | 696.05 | 696.05 | 695.90 | 695.96 | 696.04 | | | 3,4 |
| 75-73-0 | tetrafluoromethane | $CF_4$ | C1s | 301.90 | 302.29 | 302.32 | 302.50 | 302.62 | 0.96 | 0.07 | 3-6 |
| 593-53-3 | fluoromethane | $CH_3F$ | F1s | 693.34 | 693.34 | 693.26 | 693.32 | 693.33 | | | 3,4 |
| 593-53-3 | fluoromethane | $CH_3F$ | C1s | 294.25 | 294.55 | 294.64 | 294.87 | 294.92 | 0.94 | 0.07 | 3-6 |
| 75-46-7 | trifluoromethane | $CHF_3$ | F1s | 695.16 | 695.16 | 695.08 | 695.12 | 695.16 | | | 3,4 |
| 75-46-7 | trifluoromethane | $CHF_3$ | C1s | 299.39 | 299.78 | 299.88 | 300.08 | 300.20 | 0.98 | 0.05 | 3-6 |
| 67-56-1 | methanol | $CH_3OH$ | O1s | 539.86 | 539.97 | 539.97 | 540.13 | 540.17 | 0.94 | 0.05 | 3,4,6 |
| 67-56-1 | methanol | $CH_3OH$ | C1s | 293.14 | 293.43 | 293.53 | 293.74 | 293.79 | 0.95 | 0.07 | 3-6 |
| 50-00-0 | formaldehyde | $CH_2O$ | O1s | 540.49 | 540.56 | 540.57 | 540.67 | 540.61 | 0.98 | 0.01 | 3-5 |
| 50-00-0 | formaldehyde | $CH_2O$ | C1s | 295.22 | 295.53 | 295.61 | 295.82 | 295.89 | 0.95 | 0.06 | 3-6 |
| 115-10-6 | dimethyl ether | $CH_3OCH_3$ | O1s | 539.42 | 539.49 | 539.53 | 539.62 | 539.57 | 1.00 | 0.00 | 3-5 |
| 115-10-6 | dimethyl ether | $CH_3OCH_3$ | C1s | 292.90 | 293.19 | 293.28 | 293.48 | 293.53 | 0.94 | 0.06 | 3-6 |

† spin-polarized $G_{RS}W_{RS}$ calculations not available in QM4E

**Table S3:** Continued

| CAS | name | formula | core level | evGW@PBE $n=3$ | $n=4$ | $n=5$ | $n=6$ | ∞ | SE | $R^2$ | $n$ used |
|---|---|---|---|---|---|---|---|---|---|---|---|
| 64-18-6 | formic acid | HCOOH | O1s (OH) | 541.55 | 541.66 | 541.69 | 541.84 | 541.76 | 1.00 | 0.01 | 3-5 |
| 64-18-6 | formic acid | HCOOH | O1s (C=O) | 539.80 | 539.91 | 539.96 | 540.08 | 540.10 | 0.90 | 0.04 | 3-6 |
| 64-18-6 | formic acid | HCOOH | C1s | 296.09 | 296.44 | 296.54 | 296.75 | 296.84 | 0.96 | 0.06 | 3-6 |
| 67-64-1 | acetone | $(CH_3)_2CO$ | O1s | 538.77 | 538.88 | 538.92 | 539.03 | 538.99 | 1.00 | 0.01 | 3-5 |
| 67-64-1 | acetone | $(CH_3)_2CO$ | C1s (C=O) | 294.26 | 294.54 | 294.64 | 294.84 | 294.89 | 0.95 | 0.06 | 3-6 |
| 67-64-1 | acetone | $(CH_3)_2CO$ | C1s ($CH_3$) | 291.84 | 292.12 | 292.21 | 292.42 | 292.46 | 0.94 | 0.07 | 3-6 |
| 107-31-3 | methyl formate | $HCO_2CH_3$ | O1s ($OCH_3$) | 540.83 | 540.92 | 540.99 | 541.11 | 541.05 | 0.98 | 0.02 | 3-5 |
| 107-31-3 | methyl formate | $HCO_2CH_3$ | O1s (C=O) | 539.31 | 539.43 | 539.50 | 539.62 | 539.64 | 0.90 | 0.05 | 3-6 |
| 64-19-7 | acetic acid | $CH_3COOH$ | O1s (OH) | 540.89 | 541.02 | 541.06 | 541.20 | 541.15 | 0.99 | 0.01 | 3-5 |
| 64-19-7 | acetic acid | $CH_3COOH$ | O1s (C=O) | 539.01 | 539.15 | 539.22 | 539.34 | 539.36 | 0.92 | 0.04 | 3-6 |
| 64-19-7 | acetic acid | $CH_3COOH$ | C1s (COOH) | 295.61 | 295.96 | 296.07 | 296.27 | 296.36 | 0.97 | 0.06 | 3-6 |
| 64-19-7 | acetic acid | $CH_3COOH$ | C1s ($CH_3$) | 292.23 | 292.53 | 292.61 | 292.83 | 292.88 | 0.94 | 0.07 | 3-6 |
| 7732-18-5 | water | $H_2O$ | O1s | 540.67 | 540.80 | 540.79 | 540.96 | 541.00 | 0.98 | 0.04 | 3,4,6 |
| 10028-15-6 | ozone | $O_3$ | O1s middle | 548.05 | 548.16 | 548.18 | 548.29 | 548.35 | 0.98 | 0.03 | 3,4,6 |
| 10028-15-6 | ozone | $O_3$ | O1s terminal | 542.92 | 542.97 | 542.97 | 543.07 | 543.03 | | | 3,4 |
| 7782-44-7 | oxygen | $O_2$ | O1s weaker | 545.61 | 545.65 | 545.55 | 545.68 | 545.70 | 1.00 | 0.00 | 3,4,6 |
| 7782-44-7 | oxygen | $O_2$ | O1s stronger | 544.48 | 544.53 | 544.49 | 544.60 | 544.59 | | | 3,4 |
| 7727-37-9 | nitrogen | $N_2$ | N1s | 410.75 | 410.96 | 410.99 | 411.12 | 411.18 | 0.95 | 0.04 | 3-6 |
| 7664-41-7 | ammonia | $NH_3$ | N1s | 406.32 | 406.66 | 406.75 | 406.89 | 406.98 | 0.99 | 0.03 | 3-6 |
| 74-90-8 | hydrogen cyanide | HCN | N1s | 407.76 | 408.02 | 408.06 | 408.26 | 408.31 | 0.92 | 0.07 | 3-6 |
| 74-90-8 | hydrogen cyanide | HCN | C1s | 294.13 | 294.35 | 294.45 | 294.64 | 294.69 | 0.93 | 0.07 | 3-6 |
| 75-05-8 | acetonitrile | $CH_3CN$ | N1s | 406.48 | 406.74 | 406.80 | 406.95 | 407.02 | 0.96 | 0.05 | 3-6 |
| 75-05-8 | acetonitrile | $CH_3CN$ | C1s ($CH_3$) | 293.40 | 293.67 | 293.75 | 293.96 | 294.01 | 0.93 | 0.07 | 3-6 |
| 75-05-8 | acetonitrile | $CH_3CN$ | C1s (CN) | 293.31 | 293.56 | 293.66 | 293.87 | 293.91 | 0.93 | 0.07 | 3-6 |
| 56-40-6 | glycine | $C_2H_5NO_2$ | O1s (OH) | 540.88 | 541.03 | 541.09 | 541.24 | 541.25 | 0.90 | 0.05 | 3-6 |
| 56-40-6 | glycine | $C_2H_5NO_2$ | O1s (C=O) | 539.10 | 539.24 | 539.34 | 539.47 | 539.50 | 0.93 | 0.05 | 3-6 |
| 56-40-6 | glycine | $C_2H_5NO_2$ | N1s | 406.18 | 406.47 | 406.55 | 406.77 | 406.82 | 0.93 | 0.07 | 3-6 |
| 56-40-6 | glycine | $C_2H_5NO_2$ | C1s (COOH) | 295.39 | 295.75 | 295.88 | 296.09 | 296.18 | 0.97 | 0.06 | 3-6 |
| 56-40-6 | glycine | $C_2H_5NO_2$ | C1s ($CH_2$) | 292.84 | 293.18 | 293.28 | 293.50 | 293.58 | 0.96 | 0.07 | 3-6 |
| 110-86-1 | pyridine | $C_5H_5N$ | N1s | 405.58 | 405.76 | 405.88 | 406.03 | 406.07 | 0.94 | 0.06 | 3-6 |
| 109-97-7 | pyrrole | $C_4H_4NH$ | N1s | 406.98 | 407.22 | 407.36 | 407.55 | 407.60 | 0.94 | 0.07 | 3-6 |
| 62-53-3 | aniline | $C_6H_5NH_2$ | N1s | 405.96 | 406.21 | 406.37 | 406.56 | 406.62 | 0.94 | 0.07 | 3-6 |
| 57-13-6 | urea | $CO(NH_2)_2$ | O1s | 537.86 | 538.01 | 538.08 | 538.22 | 538.24 | 0.92 | 0.05 | 3-6 |
| 57-13-6 | urea | $CO(NH_2)_2$ | N1s | 406.76 | 407.08 | 407.18 | 407.38 | 407.46 | 0.96 | 0.06 | 3-6 |
| 57-13-6 | urea | $CO(NH_2)_2$ | C1s | 295.06 | 295.42 | 295.55 | 295.77 | 295.86 | 0.97 | 0.06 | 3-6 |
| 74-89-5 | methylamine | $CH_3NH_2$ | N1s | 406.04 | 406.19 | 406.26 | 406.44 | 406.35 | 1.00 | 0.00 | 3-5 |
| 98-95-3 | nitrobenzene | $C_6H_5NO_2$ | O1s | 539.46 | 539.60 | 539.65 | * | 539.74 | 0.99 | 0.01 | 3-5 |
| 98-95-3 | nitrobenzene | $C_6H_5NO_2$ | N1s | 412.15 | 412.44 | 412.58 | * | 412.78 | 1.00 | 0.00 | 3-5 |
| 98-95-3 | nitrobenzene | $C_6H_5NO_2$ | C1s (C1) | 292.67 | 292.94 | 293.09 | * | 293.27 | 1.00 | 0.02 | 3-5 |
| 98-95-3 | nitrobenzene | $C_6H_5NO_2$ | C1s (C2-4) | 291.82 | 292.10 | 292.24 | * | 292.42 | 1.00 | 0.01 | 3-5 |
| 71-43-2 | benzene | $C_6H_6$ | C1s | 291.09 | 291.33 | 291.48 | 291.67 | 291.73 | 0.94 | 0.07 | 3-6 |
| 536-74-3 | phenylacetylene | $C_8H_6$ | C1s (C3) | 291.76 | 292.02 | 292.12 | 292.31 | 292.37 | 0.94 | 0.06 | 3-6 |
| 536-74-3 | phenylacetylene | $C_8H_6$ | C1s (C2) | 291.34 | 291.59 | 291.67 | 291.89 | 291.93 | 0.92 | 0.08 | 3-6 |
| 536-74-3 | phenylacetylene | $C_8H_6$ | C1s (C4-6) | 291.20 | 291.47 | 291.56 | 291.76 | 291.82 | 0.95 | 0.06 | 3-6 |
| 536-74-3 | phenylacetylene | $C_8H_6$ | C1s (C1) | 290.94 | 291.24 | 291.27 | 291.51 | 291.55 | 0.91 | 0.08 | 3-6 |

* ev*GW* outer cycle not converged

# 3 $G_{\Delta H}W_0$ results without relativistic correction

**Table S4:** Non-relativistic core-level binding energies from $G_{\Delta H}W_0$@PBE using the cc-pV$n$Z basis set series with $n = 3 - 6$. Extrapolated values ($\infty$), standard error (SE) and correlation coefficient $R^2$. The last column indicates the basis sets used for the extrapolation; for most cases all data points ($n = 3-6$) are included; see SI of Ref. 1 for a discussion why $n = 5, 6$ are sometimes excluded. All values in eV.

| | | | | $G_{\Delta H}W_0$@PBE | | | | | | | |
|---|---|---|---|---|---|---|---|---|---|---|---|
| CAS | name | formula | core level | $n = 3$ | $n = 4$ | $n = 5$ | $n = 6$ | $\infty$ | SE | $R^2$ | $n$ used |
| 74-82-8 | methane | $CH_4$ | C1s | 290.00 | 290.27 | 290.39 | 290.44 | 290.53 | 1.00 | 0.00 | 3-6 |
| 74-84-0 | ethane | $C_2H_6$ | C1s | 289.89 | 290.20 | 290.25 | 290.53 | 290.63 | 0.98 | 0.07 | 3,4,6 |
| 74-85-1 | ethene | $C_2H_4$ | C1s | 290.10 | 290.41 | 290.45 | 290.71 | 290.74 | 0.90 | 0.09 | 3-6 |
| 74-86-2 | ethyne | $C_2H_2$ | C1s | 290.50 | 290.76 | 290.93 | 291.21 | 291.10 | 0.99 | 0.04 | 3-5 |
| 630-08-0 | carbon monoxide | CO | O1s | 541.44 | 541.53 | 541.41 | 541.67 | 541.72 | 0.97 | 0.04 | 3,4,6 |
| 630-08-0 | carbon monoxide | CO | C1s | 295.15 | 295.38 | 295.48 | 295.65 | 295.72 | 0.95 | 0.06 | 3-6 |
| 124-38-9 | carbon dioxide | $CO_2$ | O1s | 540.15 | 540.28 | 540.33 | 540.51 | 540.42 | 1.00 | 0.01 | 3-5 |
| 124-38-9 | carbon dioxide | $CO_2$ | C1s | 296.26 | 296.22 | 296.85 | 296.96 | 297.14 | 1.00 | 0.00 | 3,5,6 |
| 75-73-0 | tetrafluoromethane | $CF_4$ | F1s | 693.61 | 693.64 | 693.62 | 693.79 | 693.81 | 0.81 | 0.07 | 3,4,6 |
| 75-73-0 | tetrafluoromethane | $CF_4$ | C1s | 300.16 | 300.63 | 300.75 | 300.97 | 301.13 | 0.98 | 0.06 | 3-6 |
| 593-53-3 | fluoromethane | $CH_3F$ | F1s | 691.23 | 691.24 | 691.20 | 691.21 | 691.26 | | | 3,4 |
| 593-53-3 | fluoromethane | $CH_3F$ | C1s | 292.57 | 292.99 | 293.08 | 293.34 | 293.42 | 0.95 | 0.08 | 3-6 |
| 75-46-7 | trifluoromethane | $CHF_3$ | F1s | 692.80 | 692.84 | 692.81 | 692.91 | 692.88 | | | 3,4 |
| 75-46-7 | trifluoromethane | $CHF_3$ | C1s | 297.69 | 298.15 | 298.26 | 298.51 | 298.65 | 0.97 | 0.07 | 3-6 |
| 67-56-1 | methanol | $CH_3OH$ | O1s | 537.96 | 538.09 | 538.06 | 538.40 | 538.22 | | | 3,4 |
| 67-56-1 | methanol | $CH_3OH$ | C1s | 291.53 | 291.87 | 291.99 | 292.27 | 292.32 | 0.93 | 0.09 | 3-6 |
| 50-00-0 | formaldehyde | $CH_2O$ | O1s | 538.36 | 538.48 | 538.35 | 538.73 | 538.61 | | | 3,4 |
| 50-00-0 | formaldehyde | $CH_2O$ | C1s | 293.60 | 293.95 | 294.06 | 294.34 | 294.40 | 0.93 | 0.09 | 3-6 |
| 115-10-6 | dimethyl ether | $CH_3OCH_3$ | O1s | 537.51 | 537.61 | 537.72 | 537.83 | 537.84 | 0.90 | 0.05 | 3-6 |
| 115-10-6 | dimethyl ether | $CH_3OCH_3$ | C1s | 291.32 | 291.66 | 291.77 | 292.03 | 292.08 | 0.94 | 0.08 | 3-6 |
| 64-18-6 | formic acid | HCOOH | O1s (OH) | 539.47 | 539.62 | 539.66 | 539.80 | 539.82 | 0.91 | 0.05 | 3-6 |
| 64-18-6 | formic acid | HCOOH | O1s (C=O) | 537.65 | 537.80 | 537.63 | 538.02 | 538.08 | 0.95 | 0.07 | 3,4,6 |
| 64-18-6 | formic acid | HCOOH | C1s | 294.50 | 294.89 | 295.01 | 295.24 | 295.34 | 0.97 | 0.07 | 3-6 |
| 67-64-1 | acetone | $(CH_3)_2CO$ | O1s | 536.69 | 536.83 | 536.66 | 537.05 | 537.10 | 0.93 | 0.08 | 3,4,6 |
| 67-64-1 | acetone | $(CH_3)_2CO$ | C1s (C=O) | 292.55 | 293.03 | 293.17 | 293.37 | 293.50 | 0.99 | 0.05 | 3-6 |
| 67-64-1 | acetone | $(CH_3)_2CO$ | C1s ($CH_3$) | 290.27 | 290.60 | 290.67 | 290.92 | 290.97 | 0.93 | 0.08 | 3-6 |
| 107-31-3 | methyl formate | $HCO_2CH_3$ | O1s ($OCH_3$) | 538.79 | 538.92 | 539.04 | 539.12 | 539.16 | 0.95 | 0.03 | 3-6 |
| 107-31-3 | methyl formate | $HCO_2CH_3$ | O1s (C=O) | 537.19 | 537.34 | 537.29 | 537.52 | 537.58 | 0.97 | 0.04 | 3,4,6 |
| 64-19-7 | acetic acid | $CH_3COOH$ | O1s (OH) | 538.87 | 539.03 | 539.00 | 539.25 | 539.31 | 0.96 | 0.06 | 3,4,6 |
| 64-19-7 | acetic acid | $CH_3COOH$ | O1s (C=O) | 536.93 | 537.08 | 536.99 | 537.28 | 537.34 | 0.97 | 0.05 | 3,4,6 |
| 64-19-7 | acetic acid | $CH_3COOH$ | C1s (COOH) | 294.05 | 294.42 | 294.58 | 294.80 | 294.89 | 0.97 | 0.06 | 3-6 |
| 64-19-7 | acetic acid | $CH_3COOH$ | C1s ($CH_3$) | 290.65 | 290.98 | 291.08 | 291.33 | 291.39 | 0.94 | 0.08 | 3-6 |
| 7732-18-5 | water | $H_2O$ | O1s | 538.68 | 538.83 | 538.75 | 538.97 | 539.02 | 0.99 | 0.02 | 3,4,6 |
| 10028-15-6 | ozone | $O_3$ | O1s middle | 545.91 | 546.04 | 546.01 | 546.30 | 546.37 | 0.93 | 0.09 | 3,4,6 |
| 10028-15-6 | ozone | $O_3$ | O1s terminal | 540.63 | 540.71 | 540.75 | 540.88 | 540.80 | 1.00 | 0.00 | 3-5 |
| 7782-44-7 | oxygen | $O_2$ | O1s weaker | 543.18 | 543.23 | 543.30 | 543.37 | 543.34 | 0.91 | 0.04 | 3-5 |
| 7782-44-7 | oxygen | $O_2$ | O1s stronger | 542.28 | 542.33 | 542.41 | 542.50 | 542.45 | 0.92 | 0.04 | 3-5 |
| 7727-37-9 | nitrogen | $N_2$ | N1s | 408.89 | 408.87 | 409.13 | 409.36 | 409.64 | 0.98 | 0.08 | 4,5,6 |
| 7664-41-7 | ammonia | $NH_3$ | N1s | 404.47 | 404.98 | 405.02 | 405.15 | 405.30 | 0.96 | 0.07 | 3-6 |
| 74-90-8 | hydrogen cyanide | HCN | N1s | 405.85 | 406.10 | 406.12 | 406.34 | 406.45 | 0.99 | 0.04 | 3,4,6 |
| 74-90-8 | hydrogen cyanide | HCN | C1s | 292.55 | 292.78 | 293.00 | 293.12 | 293.22 | 0.97 | 0.06 | 3-6 |
| 75-05-8 | acetonitrile | $CH_3CN$ | N1s | 404.57 | 404.84 | 404.90 | 405.08 | 405.14 | 0.95 | 0.05 | 3-6 |
| 75-05-8 | acetonitrile | $CH_3CN$ | C1s ($CH_3$) | 291.82 | 292.16 | 292.23 | 292.60 | 292.44 | 0.98 | 0.06 | 3-5 |
| 75-05-8 | acetonitrile | $CH_3CN$ | C1s (CN) | 291.77 | 291.97 | 292.12 | 292.36 | 292.25 | 0.99 | 0.04 | 3-5 |

**Table S4:** Continued

| CAS | name | formula | core level | $G_{\Delta H}W_0$@PBE | | | | | SE | $R^2$ | $n$ used |
|---|---|---|---|---|---|---|---|---|---|---|---|
| | | | | $n = 3$ | $n = 4$ | $n = 5$ | $n = 6$ | $\infty$ | | | |
| 56-40-6 | glycine | $C_2H_5NO_2$ | O1s (OH) | 538.88 | 539.05 | 539.12 | 539.26 | 539.29 | 0.93 | 0.05 | 3-6 |
| 56-40-6 | glycine | $C_2H_5NO_2$ | O1s (C=O) | 537.00 | 537.16 | 537.35 | 537.37 | 537.46 | 0.95 | 0.04 | 3-6 |
| 56-40-6 | glycine | $C_2H_5NO_2$ | N1s | 404.62 | 404.77 | 404.87 | 405.07 | 404.96 | 0.99 | 0.02 | 3-5 |
| 56-40-6 | glycine | $C_2H_5NO_2$ | C1s (COOH) | 293.80 | 294.21 | 294.38 | 294.59 | 294.71 | 0.98 | 0.05 | 3-6 |
| 56-40-6 | glycine | $C_2H_5NO_2$ | C1s ($CH_2$) | 291.29 | 291.63 | 291.77 | 292.02 | 292.09 | 0.95 | 0.08 | 3-6 |
| 110-86-1 | pyridine | $C_5H_5N$ | N1s | 403.89 | 404.06 | 404.22 | 404.39 | 404.43 | 0.91 | 0.08 | 3-6 |
| 109-97-7 | pyrrole | $C_4H_4NH$ | N1s | 404.85 | 405.54 | 405.59 | 405.80 | 406.01 | 0.96 | 0.10 | 3-6 |
| 62-53-3 | aniline | $C_6H_5NH_2$ | N1s | 404.30 | 404.53 | 404.61 | 404.83 | 404.86 | 0.91 | 0.08 | 3-6 |
| 57-13-6 | urea | $CO(NH_2)_2$ | O1s | 535.77 | 535.95 | 535.78 | 536.18 | 536.25 | 0.96 | 0.06 | 3,4,6 |
| 57-13-6 | urea | $CO(NH_2)_2$ | N1s | 405.02 | 405.31 | 405.46 | 405.61 | 405.70 | 0.98 | 0.04 | 3-6 |
| 57-13-6 | urea | $CO(NH_2)_2$ | C1s | 293.61 | 293.94 | 294.07 | 294.31 | 294.37 | 0.95 | 0.08 | 3-6 |
| 74-89-5 | methylamine | $CH_3NH_2$ | N1s | 404.35 | 404.52 | 404.61 | 404.80 | 404.70 | 1.00 | 0.01 | 3-5 |
| 98-95-3 | nitrobenzene | $C_6H_5NO_2$ | O1s | 537.34 | 537.48 | 537.61 | 537.71 | 537.76 | 0.94 | 0.04 | 3-6 |
| 98-95-3 | nitrobenzene | $C_6H_5NO_2$ | N1s | 410.36 | 410.79 | 410.74 | 411.06 | 411.24 | 1.00 | 0.01 | 3,4,6 |
| 98-95-3 | nitrobenzene | $C_6H_5NO_2$ | C1s (C1) | 291.16 | 291.41 | 291.57 | 291.81 | 291.86 | 0.93 | 0.09 | 3-6 |
| 98-95-3 | nitrobenzene | $C_6H_5NO_2$ | C1s (C2-4) | 290.23 | 290.51 | 290.67 | 290.89 | 290.97 | 0.95 | 0.07 | 3-6 |
| 71-43-2 | benzene | $C_6H_6$ | C1s | 289.49 | 289.81 | 289.97 | 290.18 | 290.26 | 0.96 | 0.07 | 3-6 |
| 536-74-3 | phenylacetylene | $C_8H_6$ | C1s (C3) | 290.18 | 290.51 | 290.62 | 290.87 | 290.94 | 0.94 | 0.08 | 3-6 |
| 536-74-3 | phenylacetylene | $C_8H_6$ | C1s (C2) | 289.71 | 290.02 | 290.15 | 290.39 | 290.46 | 0.94 | 0.08 | 3-6 |
| 536-74-3 | phenylacetylene | $C_8H_6$ | C1s (C4-6) | 289.54 | 289.84 | 289.98 | 290.21 | 290.28 | 0.94 | 0.08 | 3-6 |
| 536-74-3 | phenylacetylene | $C_8H_6$ | C1s (C1) | 289.19 | 289.46 | 289.50 | 289.81 | 289.92 | 0.97 | 0.09 | 3,4,6 |

# 4 $G_{RS}W_{RS}$ results without relativistic correction

**Table S5:** Non-relativistic core-level binding energies from $G_{RS}W_{RS}$@PBE and $G_{RS}W_{RS}$@PBE0 using the cc-pV$n$Z basis set series with $n = 3, 4$ and 2-point extrapolated values ($\infty$). For $G_{RS}W_{RS}$ calculations, the cc-pV$n$Z basis sets are treated as Cartesian Gaussian functions. All values in eV.

| CAS | name | formula | core level | $G_{RS}W_{RS}$@PBE | | | $G_{RS}W_{RS}$@PBE0 | | |
|---|---|---|---|---|---|---|---|---|---|
| | | | | $n = 3$ | $n = 4$ | $\infty$ | $n = 3$ | $n = 4$ | $\infty$ |
| 74-82-8 | methane | $CH_4$ | C1s | 293.74 | 294.22 | 294.62 | 294.06 | 294.57 | 294.99 |
| 74-84-0 | ethane | $C_2H_6$ | C1s | 293.82 | 294.23 | 294.57 | 294.14 | 294.60 | 294.98 |
| 74-85-1 | ethene | $C_2H_4$ | C1s | 294.25 | 294.58 | 294.86 | 294.55 | 294.96 | 295.31 |
| 74-86-2 | ethyne | $C_2H_2$ | C1s | 294.50 | 294.88 | 295.22 | 294.88 | 295.30 | 295.69 |
| 630-08-0 | carbon monoxide | CO | O1s | 547.06 | 547.21 | 547.35 | 547.24 | 547.42 | 547.59 |
| 630-08-0 | carbon monoxide | CO | C1s | 298.41 | 298.88 | 299.35 | 298.89 | 299.39 | 299.88 |
| 124-38-9 | carbon dioxide | $CO_2$ | O1s | 546.13 | 546.24 | 546.36 | 546.43 | 546.59 | 546.75 |
| 124-38-9 | carbon dioxide | $CO_2$ | C1s | 299.60 | 300.11 | 300.61 | 300.39 | 300.98 | 301.56 |
| 75-73-0 | tetrafluoromethane | $CF_4$ | F1s | 699.56 | 700.17 | 700.77 | 699.72 | 700.36 | 701.00 |
| 75-73-0 | tetrafluoromethane | $CF_4$ | C1s | 303.68 | 304.34 | 305.01 | 304.54 | 305.18 | 305.82 |
| 593-53-3 | fluoromethane | $CH_3F$ | F1s | 696.91 | 697.68 | 698.35 | 696.91 | 697.72 | 698.44 |
| 593-53-3 | fluoromethane | $CH_3F$ | C1s | 296.32 | 296.90 | 297.41 | 296.73 | 297.31 | 297.82 |
| 75-46-7 | trifluoromethane | $CHF_3$ | F1s | 698.57 | 699.37 | 700.14 | 698.63 | 699.52 | 700.38 |
| 75-46-7 | trifluoromethane | $CHF_3$ | C1s | 301.27 | 301.89 | 302.50 | 301.97 | 302.66 | 303.33 |
| 67-56-1 | methanol | $CH_3OH$ | O1s | 543.64 | 543.94 | 544.20 | 543.84 | 544.15 | 544.42 |
| 67-56-1 | methanol | $CH_3OH$ | C1s | 295.39 | 295.85 | 296.24 | 295.74 | 296.24 | 296.67 |
| 50-00-0 | formaldehyde | $CH_2O$ | O1s | 544.35 | 544.54 | 544.70 | 544.52 | 544.74 | 544.94 |
| 50-00-0 | formaldehyde | $CH_2O$ | C1s | 297.24 | 297.77 | 298.25 | 297.70 | 298.24 | 298.73 |

**Table S5:** Continued

| CAS | name | formula | core level | $G_{RS}W_{RS}$@PBE $n=3$ | $n=4$ | $\infty$ | $G_{RS}W_{RS}$@PBE0 $n=3$ | $n=4$ | $\infty$ |
|---|---|---|---|---|---|---|---|---|---|
| 115-10-6 | dimethyl ether | $CH_3OCH_3$ | O1s | 543.62 | 543.85 | 544.06 | 543.76 | 544.02 | 544.24 |
| 115-10-6 | dimethyl ether | $CH_3OCH_3$ | C1s | 295.29 | 295.75 | 296.15 | 295.56 | 296.13 | 296.61 |
| 64-18-6 | formic acid | HCOOH | O1s (OH) | 545.48 | 545.71 | 545.93 | 545.70 | 545.95 | 546.19 |
| 64-18-6 | formic acid | HCOOH | O1s (C=O) | 543.88 | 544.09 | 544.27 | 544.12 | 544.32 | 544.52 |
| 64-18-6 | formic acid | HCOOH | C1s | 298.18 | 298.71 | 299.21 | 298.81 | 299.37 | 299.90 |
| 67-64-1 | acetone | $(CH_3)_2CO$ | O1s | 542.78 | 543.34 | 543.83 | 542.92 | 543.59 | 544.19 |
| 67-64-1 | acetone | $(CH_3)_2CO$ | C1s (C=O) | 296.63 | 297.09 | 297.50 | 297.10 | 297.62 | 298.08 |
| 67-64-1 | acetone | $(CH_3)_2CO$ | C1s ($CH_3$) | 294.28 | 294.73 | 295.13 | 294.64 | 295.13 | 295.56 |
| 107-31-3 | methyl formate | $HCO_2CH_3$ | O1s ($OCH_3$) | 545.12 | 545.26 | 545.39 | 545.32 | 545.51 | 545.68 |
| 107-31-3 | methyl formate | $HCO_2CH_3$ | O1s (C=O) | 543.61 | 543.74 | 543.87 | 543.84 | 544.03 | 544.19 |
| 64-19-7 | acetic acid | $CH_3COOH$ | O1s (OH) | 545.01 | 545.22 | 545.42 | 545.26 | 545.51 | 545.75 |
| 64-19-7 | acetic acid | $CH_3COOH$ | O1s (C=O) | 543.28 | 543.49 | 543.69 | 543.48 | 543.77 | 544.03 |
| 64-19-7 | acetic acid | $CH_3COOH$ | C1s (COOH) | 297.90 | 298.37 | 298.81 | 298.50 | 299.05 | 299.54 |
| 64-19-7 | acetic acid | $CH_3COOH$ | C1s ($CH_3$) | 294.62 | 295.10 | 295.53 | 295.00 | 295.51 | 295.97 |
| 7732-18-5 | water | $H_2O$ | O1s | 543.92 | 544.30 | 544.63 | 544.13 | 544.52 | 544.85 |
| 10028-15-6 | ozone | $O_3$ | O1s middle | 551.82 | 551.98 | 552.15 | 552.50 | 552.69 | 552.88 |
| 10028-15-6 | ozone | $O_3$ | O1s terminal | 546.85 | 547.00 | 547.15 | 547.36 | 547.51 | 547.65 |
| 7782-44-7 | oxygen | $O_2$ | O1s weaker | | | | | | |
| 7782-44-7 | oxygen | $O_2$ | O1s stronger | | | | | | |
| 7727-37-9 | nitrogen | $N_2$ | N1s | 413.25 | 413.72 | 414.20 | 413.69 | 414.17 | 414.64 |
| 7664-41-7 | ammonia | $NH_3$ | N1s | 409.21 | 409.76 | 410.22 | 409.50 | 410.06 | 410.54 |
| 74-90-8 | hydrogen cyanide | HCN | N1s | 410.79 | 411.13 | 411.45 | 411.16 | 411.53 | 411.88 |
| 74-90-8 | hydrogen cyanide | HCN | C1s | 296.04 | 296.52 | 296.98 | 296.49 | 296.94 | 297.36 |
| 75-05-8 | acetonitrile | $CH_3CN$ | N1s | 409.55 | 410.15 | 410.68 | 409.80 | 410.58 | 411.29 |
| 75-05-8 | acetonitrile | $CH_3CN$ | C1s ($CH_3$) | 295.68 | 296.14 | 296.56 | 296.13 | 296.54 | 296.91 |
| 75-05-8 | acetonitrile | $CH_3CN$ | C1s (CN) | 295.44 | 295.87 | 296.25 | 295.89 | 296.32 | 296.70 |
| 56-40-6 | glycine | $C_2H_5NO_2$ | O1s (OH) | 545.08 | 545.32 | 545.54 | 545.36 | 545.58 | 545.77 |
| 56-40-6 | glycine | $C_2H_5NO_2$ | O1s (C=O) | 542.72 | 543.70 | 544.59 | 542.77 | 543.93 | 544.99 |
| 56-40-6 | glycine | $C_2H_5NO_2$ | N1s | 409.43 | 409.94 | 410.41 | 409.76 | 410.27 | 410.74 |
| 56-40-6 | glycine | $C_2H_5NO_2$ | C1s (COOH) | 297.69 | 298.27 | 298.81 | 298.34 | 298.93 | 299.46 |
| 56-40-6 | glycine | $C_2H_5NO_2$ | C1s ($CH_2$) | 295.19 | 295.81 | 296.37 | 295.76 | 296.23 | 296.66 |
| 110-86-1 | pyridine | $C_5H_5N$ | N1s | 409.27 | 409.71 | 410.12 | 409.63 | 410.12 | 410.58 |
| 109-97-7 | pyrrole | $C_4H_4NH$ | N1s | 410.59 | 410.99 | 411.36 | 410.91 | 411.33 | 411.70 |
| 62-53-3 | aniline | $C_6H_5NH_2$ | N1s | 409.66 | 410.05 | 410.40 | 409.93 | 410.35 | 410.73 |
| 57-13-6 | urea | $CO(NH_2)_2$ | O1s | 542.32 | 542.47 | 542.60 | 542.55 | 542.73 | 542.89 |
| 57-13-6 | urea | $CO(NH_2)_2$ | N1s | 410.13 | 410.56 | 410.95 | 410.45 | 410.94 | 411.39 |
| 57-13-6 | urea | $CO(NH_2)_2$ | C1s | 297.31 | 297.86 | 298.36 | 297.98 | 298.57 | 299.10 |
| 74-89-5 | methylamine | $CH_3NH_2$ | N1s | 409.07 | 409.58 | 410.01 | 409.36 | 409.87 | 410.31 |
| 98-95-3 | nitrobenzene | $C_6H_5NO_2$ | O1s | 544.21 | 544.38 | 544.54 | 544.58 | 544.78 | 544.97 |
| 98-95-3 | nitrobenzene | $C_6H_5NO_2$ | N1s | 415.63 | 416.07 | 416.48 | 416.46 | 416.98 | 417.47 |
| 98-95-3 | nitrobenzene | $C_6H_5NO_2$ | C1s (C1) | 295.59 | 296.00 | 296.38 | 296.04 | 296.49 | 296.91 |
| 98-95-3 | nitrobenzene | $C_6H_5NO_2$ | C1s (C2-4) | 294.76 | 295.13 | 295.48 | 295.18 | 295.59 | 295.98 |
| 71-43-2 | benzene | $C_6H_6$ | C1s | 293.91 | 294.28 | 294.62 | 294.29 | 294.75 | 295.16 |
| 536-74-3 | phenylacetylene | $C_8H_6$ | C1s (C3) | 294.58 | 294.99 | 295.37 | 295.00 | 295.43 | 295.83 |
| 536-74-3 | phenylacetylene | $C_8H_6$ | C1s (C2) | 294.07 | 294.46 | 294.83 | 294.44 | 294.89 | 295.30 |
| 536-74-3 | phenylacetylene | $C_8H_6$ | C1s (C4-6) | 294.07 | 294.46 | 294.81 | 294.48 | 294.90 | 295.29 |
| 536-74-3 | phenylacetylene | $C_8H_6$ | C1s (C1) | 293.64 | 294.22 | 294.74 | 293.92 | 294.67 | 295.36 |

**Table S6:** Non-relativistic core-level binding energies from $G_{RS}W_{RS}$@B3LYP and $G_{RS}W_{RS}$@PBEh($\alpha$=0.45) using the cc-pV$n$Z basis set series with $n = 3, 4$ and 2-point extrapolated values ($\infty$). For $G_{RS}W_{RS}$ calculations, the cc-pV$n$Z basis sets are treated as Cartesian Gaussian functions. All values in eV.

| | | | | $G_{RS}W_{RS}$@B3LYP | | | $G_{RS}W_{RS}$@PBEh($\alpha$=0.45) | | |
|---|---|---|---|---|---|---|---|---|---|
| CAS | name | formula | core level | $n = 3$ | $n = 4$ | $\infty$ | $n = 3$ | $n = 4$ | $\infty$ |
| 74-82-8 | methane | $CH_4$ | C1s | 293.83 | 294.33 | 294.73 | 294.31 | 294.90 | 295.38 |
| 74-84-0 | ethane | $C_2H_6$ | C1s | 293.89 | 294.31 | 294.66 | 294.39 | 294.92 | 295.36 |
| 74-85-1 | ethene | $C_2H_4$ | C1s | 294.34 | 294.68 | 294.99 | 294.81 | 295.33 | 295.78 |
| 74-86-2 | ethyne | $C_2H_2$ | C1s | 294.58 | 295.00 | 295.37 | 295.16 | 295.64 | 296.07 |
| 630-08-0 | carbon monoxide | CO | O1s | 546.81 | 546.96 | 547.11 | 547.37 | 547.60 | 547.83 |
| 630-08-0 | carbon monoxide | CO | C1s | 298.68 | 299.16 | 299.65 | 299.26 | 299.88 | 300.49 |
| 124-38-9 | carbon dioxide | $CO_2$ | O1s | 545.98 | 546.11 | 546.23 | 546.65 | 546.91 | 547.16 |
| 124-38-9 | carbon dioxide | $CO_2$ | C1s | 300.24 | 300.81 | 301.38 | 301.00 | 301.77 | 302.55 |
| 75-73-0 | tetrafluoromethane | $CF_4$ | F1s | 699.38 | 699.96 | 700.53 | 699.84 | 700.44 | 701.04 |
| 75-73-0 | tetrafluoromethane | $CF_4$ | C1s | 304.42 | 305.06 | 305.70 | 305.19 | 305.95 | 306.70 |
| 593-53-3 | fluoromethane | $CH_3F$ | F1s | 696.56 | 697.32 | 698.00 | 696.91 | 697.79 | 698.57 |
| 593-53-3 | fluoromethane | $CH_3F$ | C1s | 296.53 | 297.11 | 297.62 | 297.06 | 297.73 | 298.33 |
| 75-46-7 | trifluoromethane | $CHF_3$ | F1s | 698.40 | 699.22 | 700.02 | 698.66 | 699.64 | 700.59 |
| 75-46-7 | trifluoromethane | $CHF_3$ | C1s | 301.82 | 302.54 | 303.23 | 302.51 | 303.30 | 304.07 |
| 67-56-1 | methanol | $CH_3OH$ | O1s | 543.35 | 543.65 | 543.91 | 543.98 | 544.36 | 544.70 |
| 67-56-1 | methanol | $CH_3OH$ | C1s | 295.54 | 296.02 | 296.44 | 296.03 | 296.64 | 297.18 |
| 50-00-0 | formaldehyde | $CH_2O$ | O1s | 544.06 | 544.26 | 544.45 | 544.64 | 544.92 | 545.16 |
| 50-00-0 | formaldehyde | $CH_2O$ | C1s | 297.50 | 298.04 | 298.53 | 298.05 | 298.70 | 299.29 |
| 115-10-6 | dimethyl ether | $CH_3OCH_3$ | O1s | 543.23 | 543.46 | 543.66 | 543.88 | 544.20 | 544.48 |
| 115-10-6 | dimethyl ether | $CH_3OCH_3$ | C1s | 295.36 | 295.90 | 296.37 | 295.83 | 296.52 | 297.11 |
| 64-18-6 | formic acid | HCOOH | O1s (OH) | 545.23 | 545.47 | 545.69 | 545.88 | 546.20 | 546.50 |
| 64-18-6 | formic acid | HCOOH | O1s (C=O) | 543.67 | 543.86 | 544.03 | 544.29 | 544.55 | 544.79 |
| 64-18-6 | formic acid | HCOOH | C1s | 298.63 | 299.18 | 299.70 | 299.28 | 299.99 | 300.64 |
| 67-64-1 | acetone | $(CH_3)_2CO$ | O1s | 542.52 | 543.11 | 543.63 | 543.02 | 543.81 | 544.51 |
| 67-64-1 | acetone | $(CH_3)_2CO$ | C1s (C=O) | 296.83 | 297.35 | 297.81 | 297.51 | 298.13 | 298.68 |
| 67-64-1 | acetone | $(CH_3)_2CO$ | C1s ($CH_3$) | 294.38 | 294.88 | 295.33 | 294.92 | 295.50 | 296.02 |
| 107-31-3 | methyl formate | $HCO_2CH_3$ | O1s ($OCH_3$) | 544.81 | 544.96 | 545.10 | 545.47 | 545.72 | 545.96 |
| 107-31-3 | methyl formate | $HCO_2CH_3$ | O1s (C=O) | 543.38 | 543.54 | 543.68 | 544.01 | 544.26 | 544.49 |
| 64-19-7 | acetic acid | $CH_3COOH$ | O1s (OH) | 544.79 | 545.02 | 545.24 | 545.45 | 545.78 | 546.08 |
| 64-19-7 | acetic acid | $CH_3COOH$ | O1s (C=O) | 543.06 | 543.30 | 543.51 | 543.63 | 544.00 | 544.34 |
| 64-19-7 | acetic acid | $CH_3COOH$ | C1s (COOH) | 298.26 | 298.81 | 299.32 | 298.98 | 299.68 | 300.32 |
| 64-19-7 | acetic acid | $CH_3COOH$ | C1s ($CH_3$) | 294.75 | 295.25 | 295.71 | 295.29 | 295.89 | 296.43 |
| 7732-18-5 | water | $H_2O$ | O1s | 543.70 | 544.09 | 544.43 | 544.30 | 544.73 | 545.11 |
| 10028-15-6 | ozone | $O_3$ | O1s middle | 551.95 | 552.12 | 552.28 | 553.03 | 553.39 | 553.75 |
| 10028-15-6 | ozone | $O_3$ | O1s terminal | 546.93 | 547.06 | 547.19 | 547.72 | 547.96 | 548.21 |
| 7782-44-7 | oxygen | $O_2$ | O1s weaker | | | | | | |
| 7782-44-7 | oxygen | $O_2$ | O1s stronger | | | | | | |
| 7727-37-9 | nitrogen | $N_2$ | N1s | 413.34 | 413.80 | 414.27 | 414.03 | 414.60 | 415.18 |
| 7664-41-7 | ammonia | $NH_3$ | N1s | 409.11 | 409.67 | 410.15 | 409.73 | 410.37 | 410.91 |
| 74-90-8 | hydrogen cyanide | HCN | N1s | 410.75 | 411.11 | 411.45 | 411.44 | 411.91 | 412.35 |
| 74-90-8 | hydrogen cyanide | HCN | C1s | 296.05 | 296.70 | 297.31 | 296.88 | 297.35 | 297.80 |
| 75-05-8 | acetonitrile | $CH_3CN$ | N1s | 409.56 | 410.15 | 410.68 | 410.59 | 410.98 | 411.34 |
| 75-05-8 | acetonitrile | $CH_3CN$ | C1s ($CH_3$) | 295.78 | 296.27 | 296.72 | 296.40 | 296.93 | 297.42 |
| 75-05-8 | acetonitrile | $CH_3CN$ | C1s (CN) | 295.61 | 296.03 | 296.41 | 296.23 | 296.82 | 297.36 |
| 56-40-6 | glycine | $C_2H_5NO_2$ | O1s (OH) | 544.88 | 545.09 | 545.28 | 545.56 | 545.85 | 546.12 |
| 56-40-6 | glycine | $C_2H_5NO_2$ | O1s (C=O) | 542.60 | 543.46 | 544.24 | 544.92 | 544.17 | 543.49 |
| 56-40-6 | glycine | $C_2H_5NO_2$ | N1s | 409.30 | 409.81 | 410.28 | 410.00 | 410.60 | 411.14 |
| 56-40-6 | glycine | $C_2H_5NO_2$ | C1s (COOH) | 298.12 | 298.69 | 299.21 | 298.87 | 299.55 | 300.17 |
| 56-40-6 | glycine | $C_2H_5NO_2$ | C1s ($CH_2$) | 295.32 | 295.96 | 296.55 | 295.99 | 296.65 | 297.26 |

**Table S6:** Continued

| CAS | name | formula | core level | $G_{RS}W_{RS}$@B3LYP $n$ = 3 | $n$ = 4 | ∞ | $G_{RS}W_{RS}$@PBE($\alpha$=0.45) $n$ = 3 | $n$ = 4 | ∞ |
|---|---|---|---|---|---|---|---|---|---|
| 110-86-1 | pyridine | $C_5H_5N$ | N1s | 409.14 | 409.61 | 410.05 | 409.90 | 410.51 | 411.07 |
| 109-97-7 | pyrrole | $C_4H_4NH$ | N1s | 410.41 | 410.82 | 411.19 | 411.15 | 411.69 | 412.18 |
| 62-53-3 | aniline | $C_6H_5NH_2$ | N1s | 409.48 | 409.89 | 410.26 | 410.15 | 410.59 | 410.99 |
| 57-13-6 | urea | $CO(NH_2)_2$ | O1s | 542.13 | 542.26 | 542.37 | 542.72 | 542.96 | 543.17 |
| 57-13-6 | urea | $CO(NH_2)_2$ | N1s | 409.95 | 410.51 | 411.01 | 410.72 | 411.29 | 411.81 |
| 57-13-6 | urea | $CO(NH_2)_2$ | C1s | 297.77 | 298.35 | 298.89 | 298.50 | 299.25 | 299.93 |
| 74-89-5 | methylamine | $CH_3NH_2$ | N1s | 408.92 | 409.43 | 409.87 | 409.59 | 410.18 | 410.69 |
| 98-95-3 | nitrobenzene | $C_6H_5NO_2$ | O1s | 544.10 | 544.26 | 544.42 | 544.82 | 545.05 | 545.26 |
| 98-95-3 | nitrobenzene | $C_6H_5NO_2$ | N1s | 415.91 | 416.42 | 416.90 | 417.06 | 417.62 | 418.15 |
| 98-95-3 | nitrobenzene | $C_6H_5NO_2$ | C1s (C1) | 295.73 | 296.14 | 296.53 | 296.41 | 296.88 | 297.33 |
| 98-95-3 | nitrobenzene | $C_6H_5NO_2$ | C1s (C2-4) | 294.88 | 295.27 | 295.63 | 295.53 | 295.97 | 296.39 |
| 71-43-2 | benzene | $C_6H_6$ | C1s | 293.97 | 294.37 | 294.72 | 294.58 | 295.03 | 295.44 |
| 536-74-3 | phenylacetylene | $C_8H_6$ | C1s (C3) | 294.64 | 295.07 | 295.46 | 295.30 | 295.76 | 296.18 |
| 536-74-3 | phenylacetylene | $C_8H_6$ | C1s (C2) | 294.14 | 294.56 | 294.95 | 294.77 | 295.22 | 295.63 |
| 536-74-3 | phenylacetylene | $C_8H_6$ | C1s (C4-6) | 294.15 | 294.56 | 294.93 | 294.79 | 295.24 | 295.66 |
| 536-74-3 | phenylacetylene | $C_8H_6$ | C1s (C1) | 293.72 | 294.31 | 294.86 | 294.58 | 295.00 | 295.39 |

# 5 ETFA molecule

**Table S7:** Core-level binding energies from different *GW* methods for the ETFA molecule using the cc-pV*n*Z basis set series with $n$ = 3 – 6. Extrapolated values (∞), extrapolated values with relativistic correction (rel. corrected), standard error (SE) and correlation coefficient $R^2$. The last column indicates the basis sets used for the extrapolation. All values in eV.

| method | core level | $n$ = 3 | $n$ = 4 | $n$ = 5 | $n$ = 6 | ∞ | rel. corrected | SE | $R^2$ | $n$ used |
|---|---|---|---|---|---|---|---|---|---|---|
| $G_0W_0$@PBEh | C1s (C1) | 298.73 | 299.03 | 299.12 | 299.29 | 299.37 | 299.49 | 0.05 | 0.97 | 3-6 |
| | C1s (C2) | 295.64 | 295.91 | 295.99 | 296.15 | 296.23 | 296.34 | 0.05 | 0.97 | 3-6 |
| | C1s (C3) | 292.82 | 293.06 | 293.14 | 293.31 | 293.37 | 293.49 | 0.05 | 0.95 | 3-6 |
| | C1s (C4) | 290.97 | 291.20 | 291.29 | 291.45 | 291.51 | 291.63 | 0.05 | 0.95 | 3-6 |
| $G_{\Delta H}W_0$@PBE | C1s (C1) | 297.38 | 297.81 | 297.94 | 298.15 | 298.28 | 298.40 | 0.05 | 0.98 | 3-6 |
| | C1s (C2) | 294.42 | 294.77 | 294.93 | 295.14 | 295.24 | 295.36 | 0.07 | 0.97 | 3-6 |
| | C1s (C3) | 292.18 | 292.52 | 292.64 | 292.90 | 292.98 | 293.09 | 0.08 | 0.95 | 3-6 |
| | C1s (C4) | 290.58 | 290.91 | 291.01 | 291.26 | 291.33 | 291.45 | 0.08 | 0.94 | 3-6 |
| ev$GW_0$@PBE | C1s (C1) | 297.20 | 297.62 | 297.77 | 297.99 | 298.11 | 298.23 | 0.06 | 0.98 | 3-6 |
| | C1s (C2) | 294.32 | 294.68 | 294.82 | 295.05 | 295.14 | 295.26 | 0.07 | 0.96 | 3-6 |
| | C1s (C3) | 292.08 | 292.41 | 292.57 | 292.79 | 292.88 | 293.00 | 0.07 | 0.96 | 3-6 |
| | C1s (C4) | 290.46 | 290.76 | 290.91 | 291.17 | 291.23 | 291.35 | 0.09 | 0.93 | 3-6 |
| ev$GW$@PBE | C1s (C1) | 298.99 | 299.38 | 299.49 | * | 299.74 | 299.86 | 0.05 | 0.99 | 3-5 |
| | C1s (C2) | 296.00 | 296.36 | 296.47 | * | 296.70 | 296.81 | 0.04 | 0.99 | 3-5 |
| | C1s (C3) | 293.83 | 294.11 | 294.23 | * | 294.42 | 294.54 | 0.01 | 1.00 | 3-5 |
| | C1s (C4) | 292.20 | 292.48 | 292.57 | * | 292.75 | 292.87 | 0.03 | 0.99 | 3-5 |
| $G_{RS}W_{RS}$@PBE | C1s (C1) | 301.24 | 301.83 | – | – | 302.37 | 302.49 | – | – | 3-4 |
| | C1s (C2) | 298.38 | 298.90 | – | – | 299.38 | 299.50 | – | – | 3-4 |
| | C1s (C3) | 296.28 | 296.76 | – | – | 297.20 | 297.32 | – | – | 3-4 |
| | C1s (C4) | 294.64 | 295.08 | – | – | 295.49 | 295.61 | – | – | 3-4 |
| $G_{RS}W_{RS}$@PBE0 | C1s (C1) | 302.06 | 302.66 | – | – | 303.22 | 303.34 | – | – | 3-4 |
| | C1s (C2) | 299.12 | 299.68 | – | – | 300.21 | 300.33 | – | – | 3-4 |
| | C1s (C3) | 296.69 | 297.22 | – | – | 297.72 | 297.84 | – | – | 3-4 |
| | C1s (C4) | 294.94 | 295.42 | – | – | 295.86 | 295.98 | – | – | 3-4 |
| $G_{RS}W_{RS}$@B3LYP | C1s (C1) | 301.85 | 302.45 | – | – | 303.01 | 303.13 | – | – | 3-4 |

**Table S7:** Continued

| method | core level | $n$ = 3 | $n$ = 4 | $n$ = 5 | $n$ = 6 | ∞ | rel. corr. | SE | $R^2$ | $n$ used |
|---|---|---|---|---|---|---|---|---|---|---|
| | C1s (C2) | 298.91 | 299.45 | – | – | 299.97 | 300.09 | – | – | 3-4 |
| | C1s (C3) | 296.44 | 296.94 | – | – | 297.40 | 297.52 | – | – | 3-4 |
| | C1s (C4) | 294.70 | 295.16 | – | – | 295.58 | 295.70 | – | – | 3-4 |
| $G_{RS}W_{RS}$@PBEh($\alpha$=0.45) | C1s (C1) | 302.68 | 303.27 | – | – | 303.83 | 303.95 | – | – | 3-4 |
| | C1s (C2) | 299.65 | 300.25 | – | – | 300.81 | 300.93 | – | – | 3-4 |
| | C1s (C3) | 297.01 | 297.57 | – | – | 298.09 | 298.21 | – | – | 3-4 |
| | C1s (C4) | 295.20 | 295.70 | – | – | 296.17 | 296.29 | – | – | 3-4 |

# 6 Graphical solution from $G_{RS}W_0$@B3LYP for O1s in $H_2O$

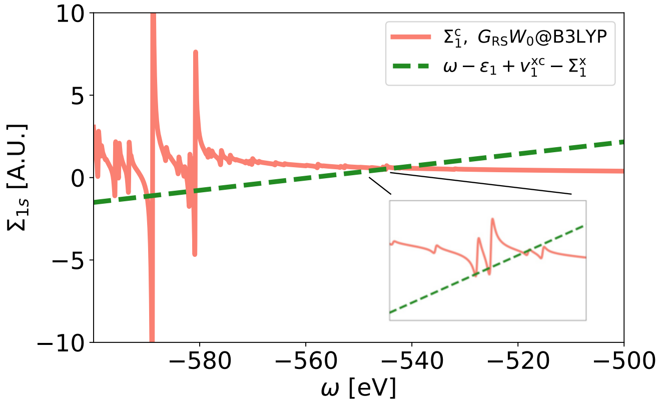


**Figure S1:** The graphical solution of O1s excitation for a single water molecule obtained from $G_{RS}W_0$@B3LYP, the cc-pVQZ basis set was used.

# 7 Errors of CLBEs and ΔCLBEs obtained from KS-DFT calculations

**Table S8:** MAEs and MEs in eV with respect to experiment for CLBEs of the CORE65 benchmark set obtained from KS-DFT eigenvalues. Calculations were performed with the QM4D package.

| | PBE | | PBE0 | | B3LYP | | PBEh | |
|---|---|---|---|---|---|---|---|---|
| | MAE | ME | MAE | ME | MAE | ME | MAE | ME |
| C1s | 22.15 | -22.15 | 12.80 | -12.80 | 14.10 | -14.10 | 2.56 | -2.56 |
| N1s | 24.88 | -24.88 | 13.95 | -13.95 | 15.72 | -15.72 | 1.79 | -1.79 |
| O1s | 27.96 | -27.96 | 15.47 | -15.47 | 17.57 | -17.57 | 1.01 | -0.94 |
| F1s | 32.39 | -32.39 | 18.35 | -18.35 | 20.72 | -20.72 | 1.62 | -1.62 |

* ev$GW$ outer cycle not converged

**Table S9:** MAEs and MEs in eV with respect to experiment for ΔCLBEs of the CORE65 benchmark set obtained from KS-DFT eigenvalues. The ΔCLBEs are the shifts with respect to a reference molecule, ΔCLBE = CLBE − $CLBE_{ref\_mol}$. $CH_4$, $NH_3$, $H_2O$ and $CH_3F$ have been used as reference molecules for C1s, N1s, O1s and F1s respectively. Calculations were performed with the QM4D package.

| | PBE | | PBE0 | | B3LYP | | PBEh | |
|---|---|---|---|---|---|---|---|---|
| | MAE | ME | MAE | ME | MAE | ME | MAE | ME |
| C1s | 0.69 | 0.13 | 0.64 | 0.28 | 0.60 | 0.26 | 0.72 | -0.22 |
| N1s | 0.68 | 0.67 | 0.75 | 0.73 | 0.68 | 0.66 | 1.16 | 1.12 |
| O1s | 1.00 | 1.16 | 1.06 | 1.14 | 0.97 | 1.07 | 1.28 | 1.26 |
| F1s | 0.23 | 0.23 | 0.16 | 0.16 | 0.15 | 0.15 | 0.13 | 0.13 |

## 8 Starting point dependence

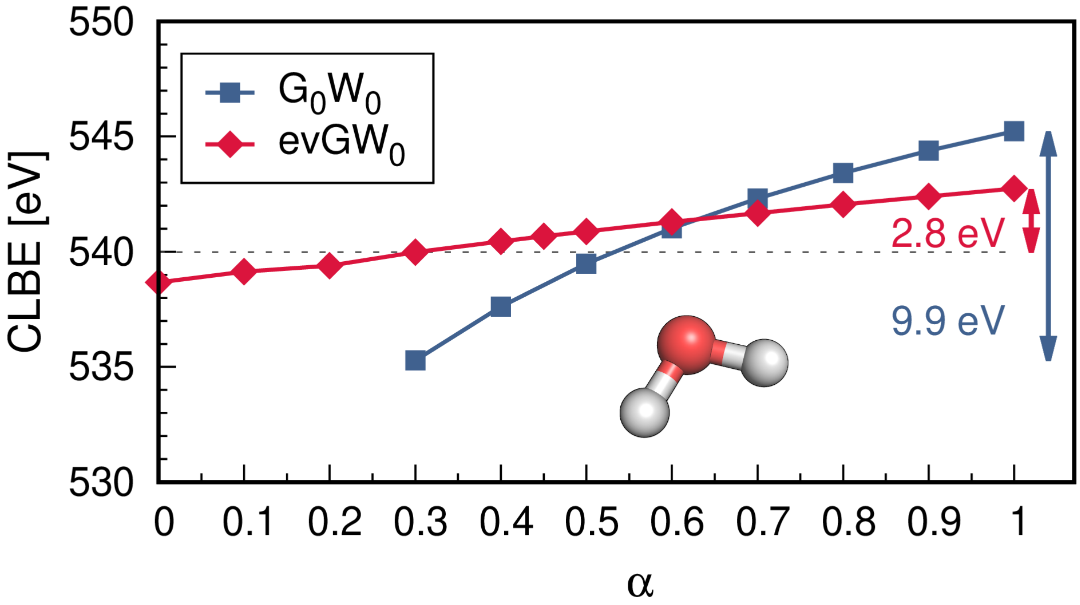


**Figure S2:** Dependence of the O1s CLBE of $H_2O$ on the amount of exact exchange $\alpha$ with $G_0W_0$@PBEh($\alpha$) and ev$GW_0$@PBEh($\alpha$). The CLBEs are obtained at the cc-pV4Z level. Relativistic corrections are not included.

# 9 ETFA geometry in xyz format

```
14

 C      1.74342172      0.79233009     -2.38607740
 C      1.87225299      0.82531137     -0.83161745
 C      1.85983154     -0.55069881      1.10298970
 C      1.77609805     -2.02516635      1.42902523
 F      1.98731130      2.01031027     -2.90139852
 F      2.61557025     -0.08958676     -2.93832354
 F      0.48395202      0.42008648     -2.74324352
 O      2.00651584      1.84892786     -0.20216186
 O      1.78925481     -0.42316165     -0.35803629
 H      2.80240352     -0.09477382      1.43702621
 H      1.02799211      0.02628227      1.53157701
 H      0.83503378     -2.45818712      1.06497140
 H      2.61261424     -2.57849042      0.98265727
 H      1.81641784     -2.15921342      2.51833177
```

# References


(1) Golze, D.; Keller, L.; Rinke, P. Accurate Absolute and Relative Core-Level Binding Energies from *GW*. *J. Phys. Chem. Lett* **2020**, *11*, 1840–1847.

(2) Keller, L.; Blum, V.; Rinke, P.; Golze, D. Relativistic correction scheme for core-level binding energies from *GW*. *J. Chem. Phys.* **2020**, *153*, 114110.
